# Supplementary material for: Bayesian modeling with spatial curvature processes
Source: arXiv:2302.05320 source file (2023-02-14)

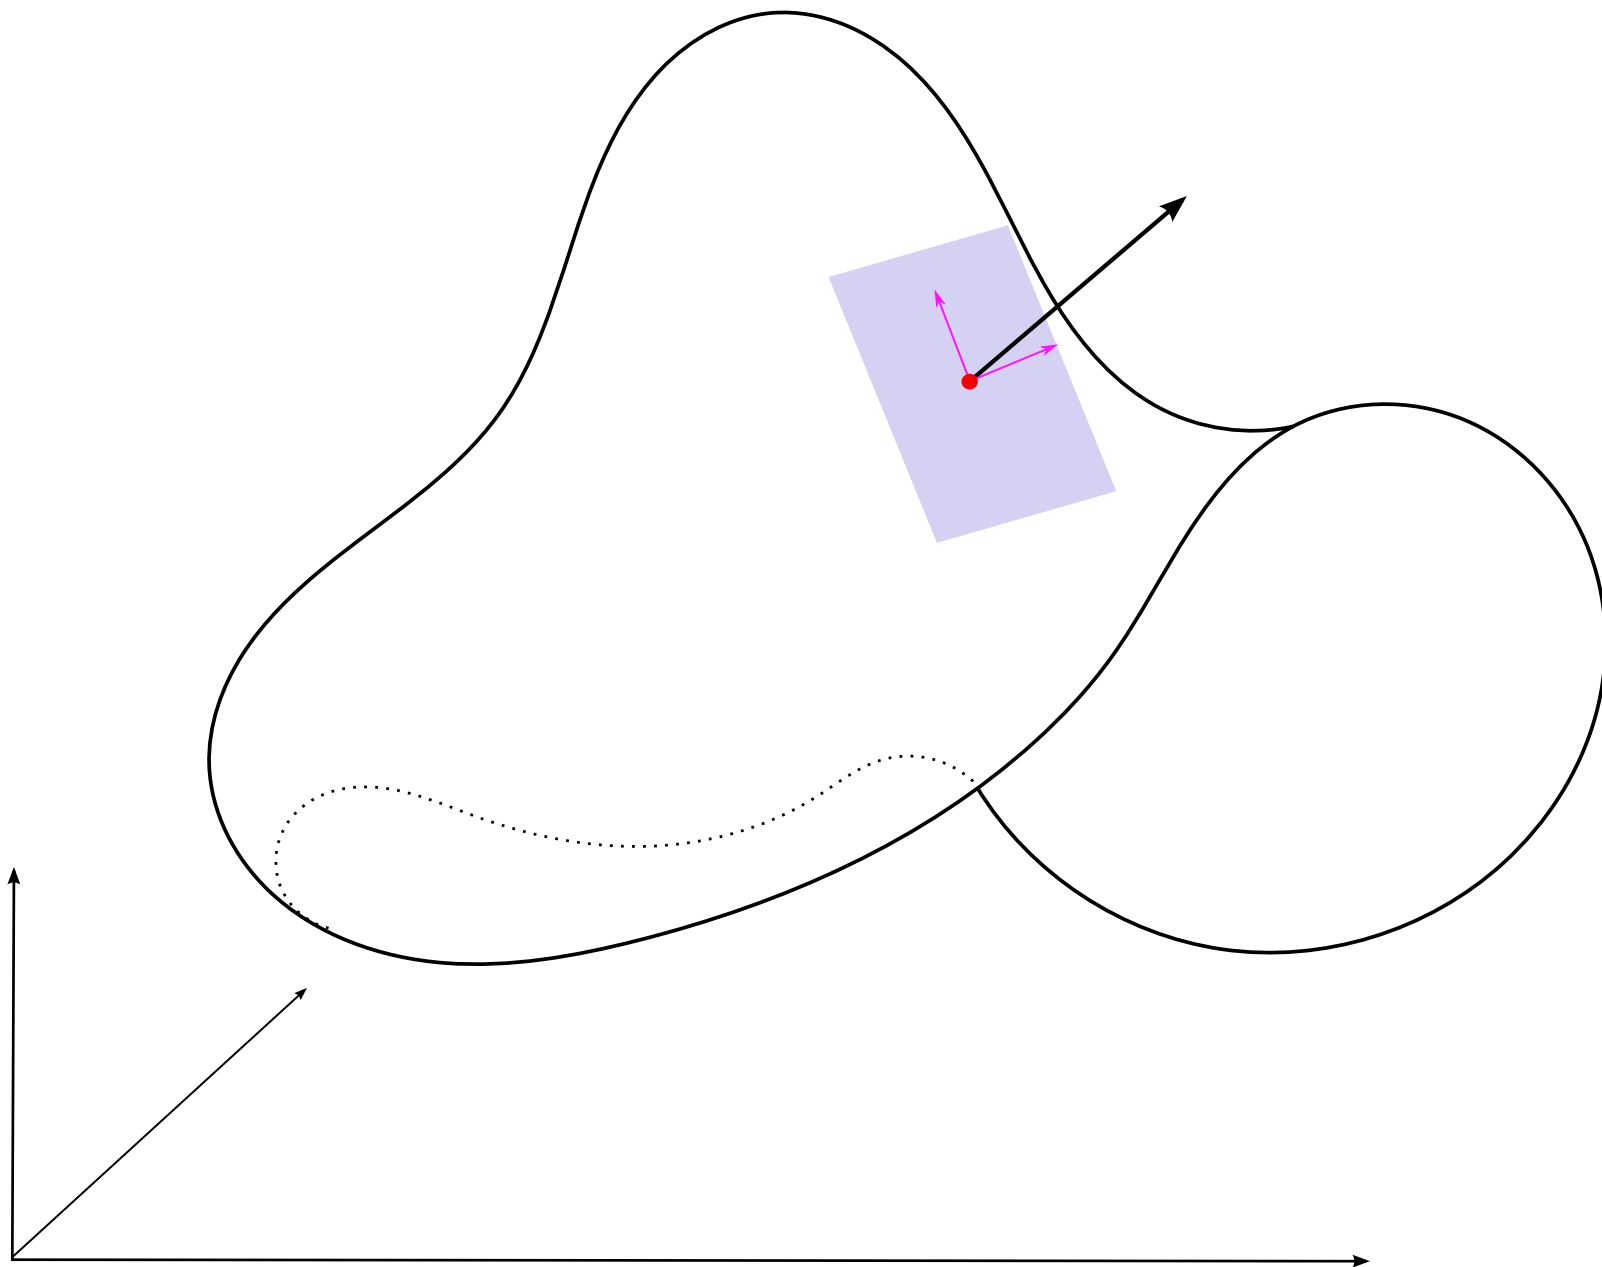

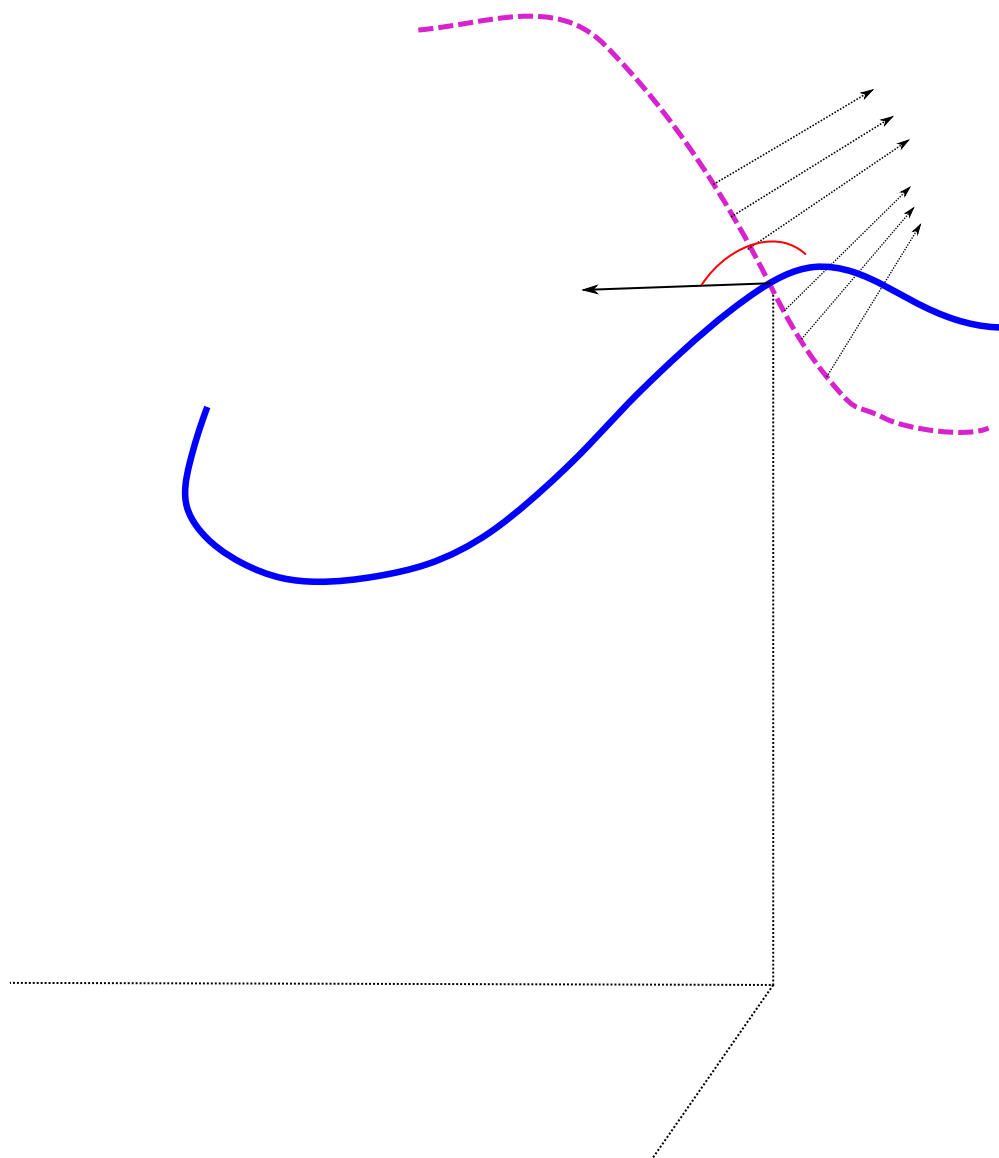

Supplement: Supplementary file 2 [file drawing-i.pdf]
