# Supplementary material for: Bayesian modeling with spatial curvature processes
Source: arXiv:2302.05320 source file (2023-02-14)

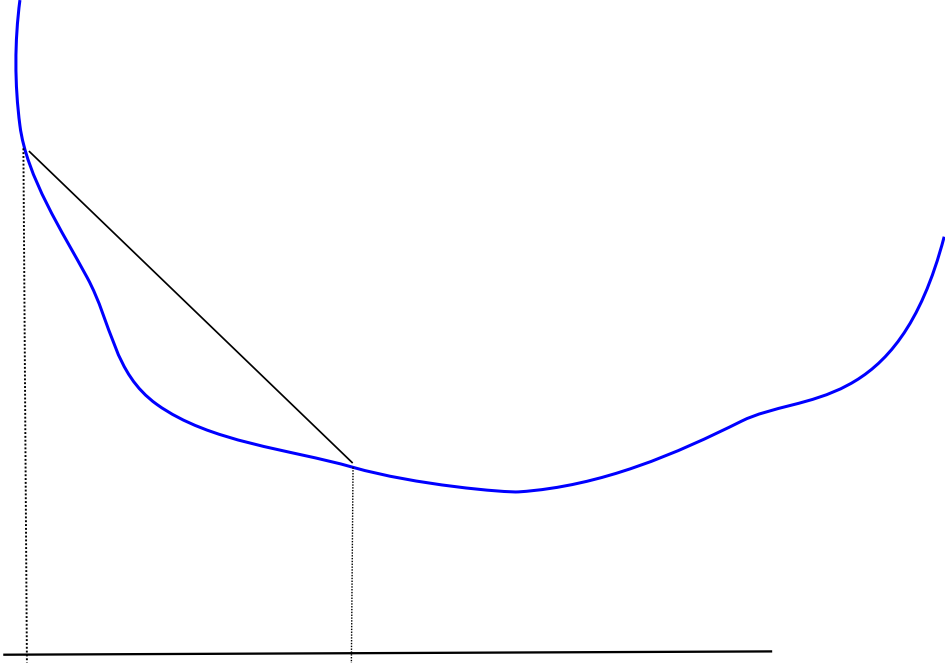

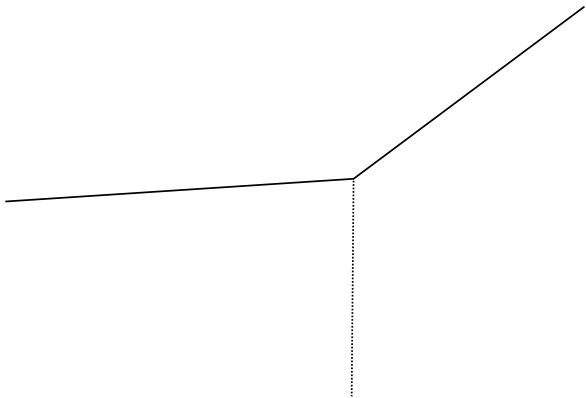

1

1

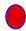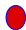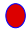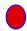

Supplement: Supplementary file 3 [file drawing-ii.pdf]
