# Supplementary material for: Bayesian modeling with spatial curvature processes
Source: arXiv:2302.05320 source file (2023-02-14)

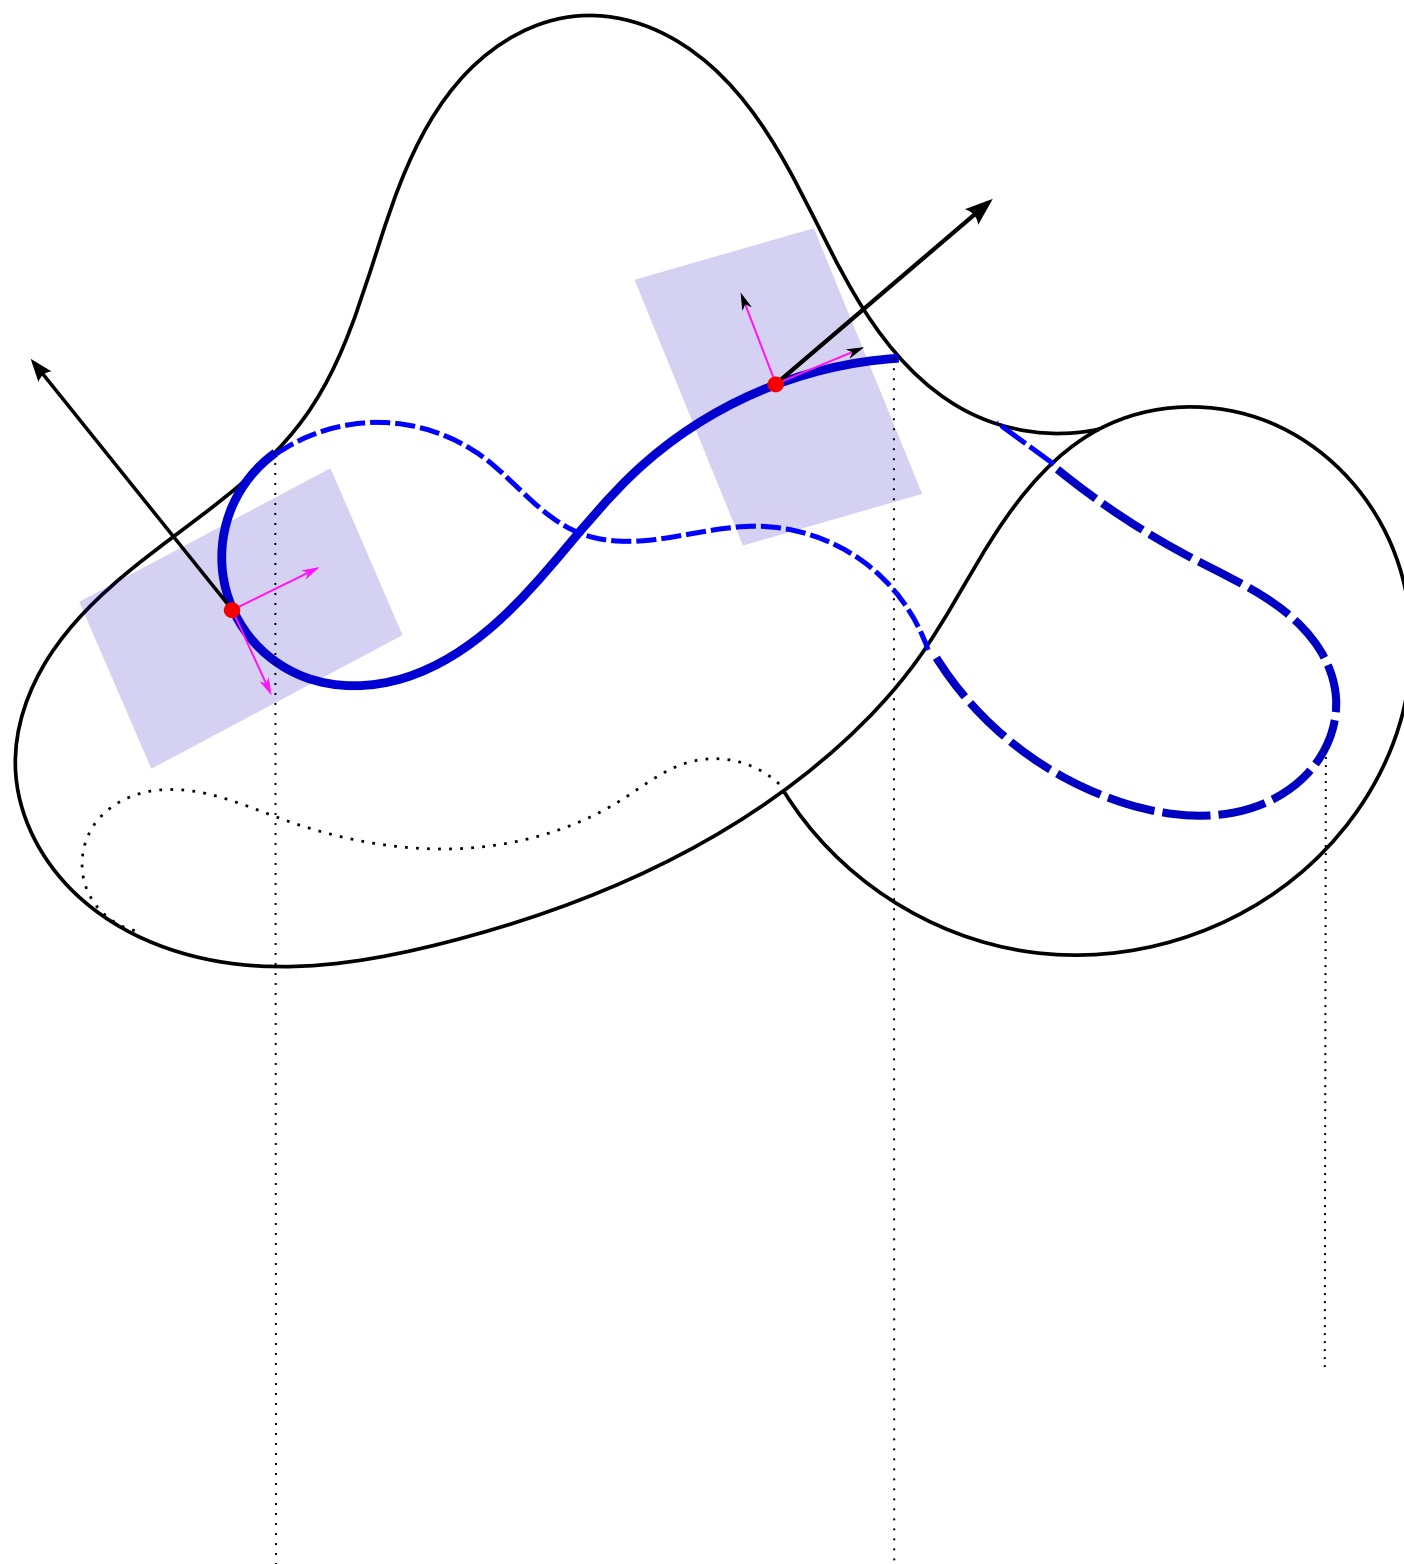

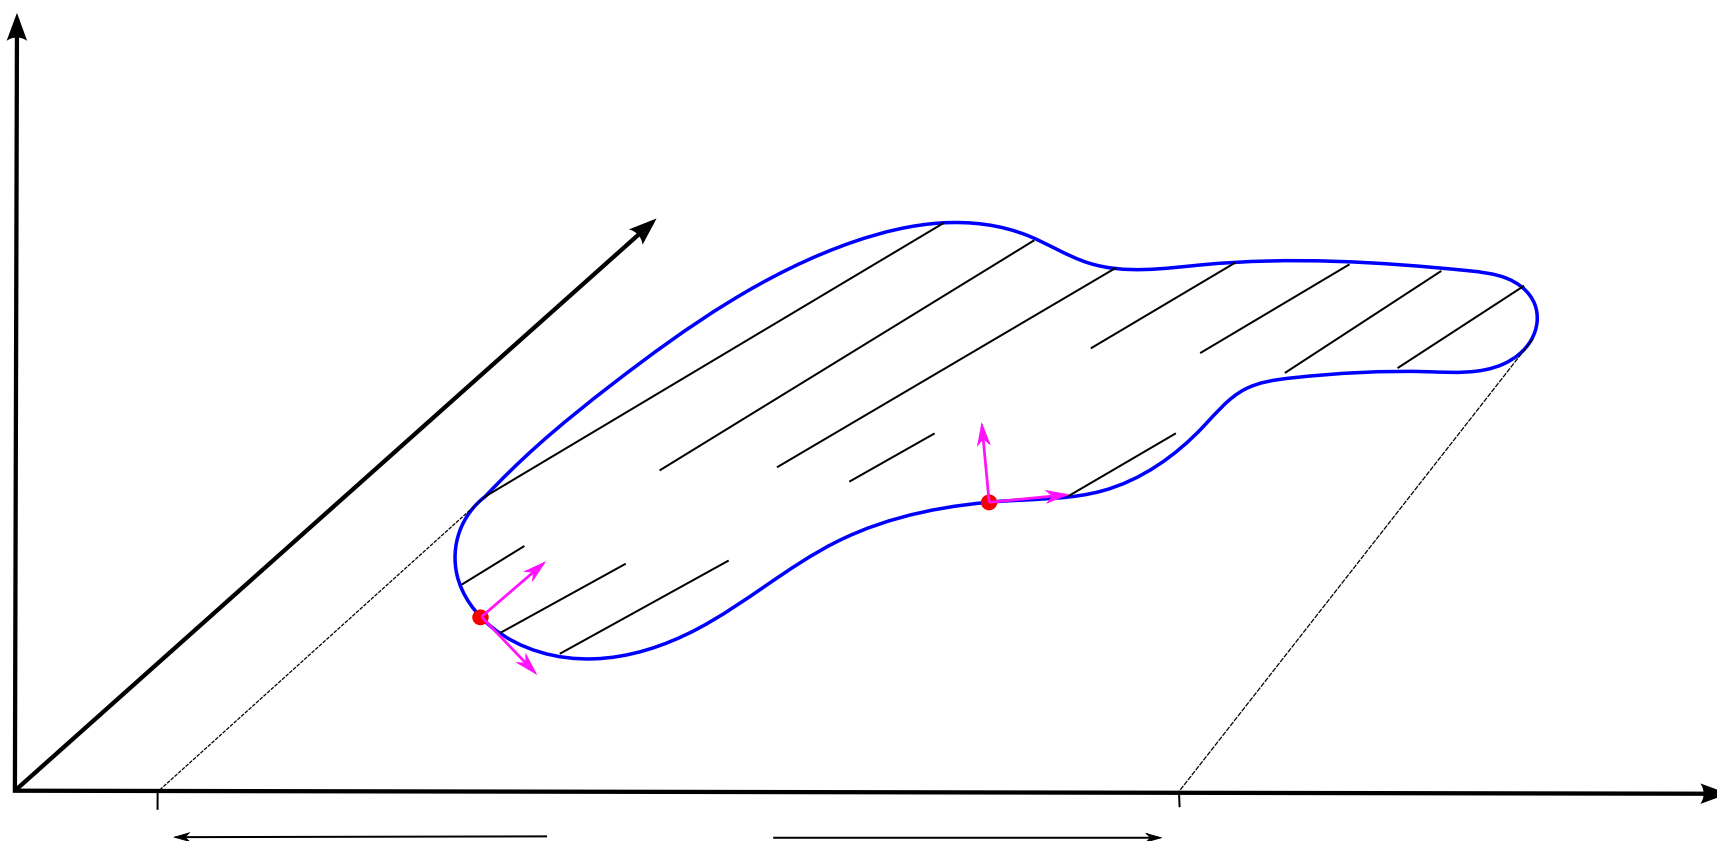

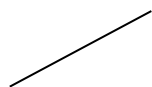

Supplement: Supplementary file 4 [file drawing.pdf]
